# Supplementary material for: Model-Predictive Control of Blood Suction for Surgical Hemostasis using Differentiable Fluid Simulations
Source: arXiv:2102.01436 source file (2021-02-02)
Supplement: Supplementary file 1 [file appendix.tex]

% \subsection{Fluid simulation details}

% \subsubsection{Detail forward simulation loop}

% Algorithm \ref{alg:detail_PBF} shows a detail PBF forward simulation loop. The mathematical details for all subroutines used in this pseudo-code are shown in the subsequent suctions. 

% \begin{algorithm}
% \caption{Detail PBF simulation loop}
% \label{alg:detail_PBF}

% \begin{algorithmic}[1]

% \FORALL{particles $i$}
%     \STATE $P'_{t,i}\leftarrow$ applyGravity($P_{t-1,i}, V_{t-1,i}, g, \Delta t)$
%     \
% \ENDFOR

% \FORALL{particles $i$}
%     \STATE find neighboring particles $N_i(X_i^*)$
% \ENDFOR

% \WHILE{iter $<$ solveIterations}

%     \FOR{\textbf{all} particles $i$}
%         \STATE calculate density constraint multiplier $\lambda_i$ using neighbor information
%     \ENDFOR
    
%     \FORALL{particles $i$}
%         \STATE calculate position correction $\Delta P_i$
%         \STATE perform collision detection
%     \ENDFOR
    
%     \FORALL{particles $i$}
%         \STATE update position $X_i^* \leftarrow X_i^* + \Delta P_i$
%     \ENDFOR
    
% \ENDWHILE

% \FORALL{particles $i$}
%     \STATE update velocity $V_i \leftarrow \frac{1}{\Delta t} (X_i^* - X_i)$
%     \STATE update position $X_i \leftarrow X_i^*$
% \ENDFOR

% \end{algorithmic}
% \end{algorithm}
